# Supplementary material for: Virtual Disk Snapshot Management at Scale
Source: arXiv:2205.06842 source file (2022-05-13)
Supplement: Supplementary file 1 [file appendix.tex]

\appendix
\section{Appendix}
\label{sec:appendix-methodo-disk-importance}

\subsection{Experimental details of Figure~\ref{fig:perfomance-slowdown}}
\begin{table}[!h]
	\scriptsize
    \centering
    \resizebox{\columnwidth}{!}
	{%
        \begin{tabular}{lcccc}
            %\toprule
            & \multicolumn{1}{c}{\textbf{Bare Metal}} & \multicolumn{1}{c}{\textbf{Virtualized}} & \multicolumn{1}{c}{\textbf{Microsoft}} & \multicolumn{1}{c}{\textbf{AWS}} \\
            & \multicolumn{1}{c}{\textbf{PC}} & \multicolumn{1}{c}{\textbf{PC}} & \multicolumn{1}{c}{\textbf{Azure}} & \multicolumn{1}{c}{\textbf{EC2}} \\
            % \midrule
            Linux / Ubuntu & 5.4.0-65-generic / & 5.4.0-65-generic / & 5.4.0-65-generic / & 5.4.0-65-generic /  \\
            versions & Ubuntu 20.04 & Ubuntu 20.04  &  Ubuntu 20.04 &  Ubuntu 18.04  \\
            \hline		
            \multirow{3}{*}{CPU} & 2 x Intel(R)  & 2 x Intel(R)  & 2 x Intel(R)  & 2 x Intel(R)  \\
             & Xeon(R) Gold  & Xeon(R) Gold  & Xeon(R)  & Xeon(R) Platinum \\
             & 6130 CPU @ 2.10GHz  & 6130 CPU @ 2.10GHz  & E5-2676 v3 @ 2.40GHz  & 8272CL @ 2.60GHz  \\
            \hline 
            RAM &  4GB & 4GB & 4GB  & 4GB \\
            \hline
            Storage Disk size & 30G & 30G & 30G & 30G \\
            \hline
            Name & - & - & Standard\_B2s & t2.medium\\
            % \bottomrule		
        \end{tabular}
    }
	\caption{Experimental environment characteristics for evaluation results on figure~\ref{fig:perfomance-slowdown}. PC stands for Private Cloud.}
	\label{tab:perfomance-slowdown-config}
\end{table}

\begin{table}[!h]
	\scriptsize
    \centering
    \resizebox{\columnwidth}{!}
	{%
        \begin{tabular}{llllll}
            % \toprule
            Benchmark & Stream & NPB & Netperf & dd & fio \\
            % \midrule
            Metric & Memory Bandwidth & FLOPS & Latency & IO rate & IOPS  \\
            % \bottomrule		
        \end{tabular}
    }
	\caption{Metric evaluated for each benchmark.
    FLOPS is the floating point operations per second of NPB applications. 
    The latency for netperf is given in microseconds. 
    IO rate is the rate of dd IO requests.
    IOPS is the number of IO requests per seconds.}
	\label{tab:perfomance-slowdown-metrics}
\end{table}

Table~\ref{tab:perfomance-slowdown-config} summarizes the characteristics of each environment.
We tried to get as much as possible the same set-up for all the environments.
For Microsoft Azure we didn't find a virtual machine with Linux 20.04 that fits all other requirements, hence Ubuntu 18.04.
The virtualized private cloud is a virtual machine that runs inside the bare metal private cloud.
AWS EC2 and Microsoft Azure are virtual machines reserved respectively on AWS and Azure.
Table~\ref{tab:perfomance-slowdown-metrics} presents the evaluated metric for each benchmark.
Each result on figure~\ref{fig:perfomance-slowdown} is a mean of 3 runs.
